# Supplementary material for: Flat-band compactons in a two-dimensional driven-dissipative Lieb lattice
Source: arXiv:2506.03963 ancillary file (2025-06-04)
Supplement: Supplementary file 1 [file Supplementary.pdf]

# Supplementary Information: Flat-band compactons in a two-dimensional driven-dissipative Lieb lattice

Seth Lovett,[1] Paul M. Walker,[1,*] Anthony Ellul,[1] Edmund Clarke,[2] Maurice S. Skolnick,[1] and Dmitry N. Krizhanovskii[1]

[1]*School of Mathematical and Physical Sciences, University of Sheffield, S3 7RH, Sheffield, UK*

[2]*EPSRC National Epitaxy Facility, University of Sheffield, Sheffield S3 7HQ, UK*

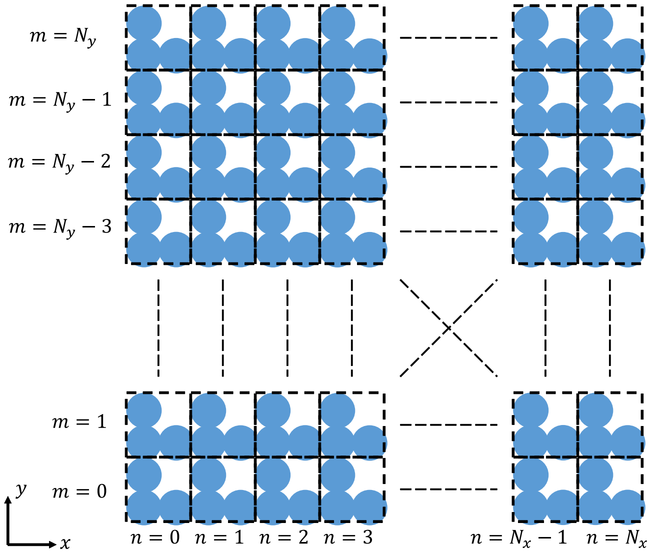


**Supplementary Figure** S1. Schematic of the simulated lattice.

## Supplementary Discussion 1. Simulation

### A. Model equations for the Lieb lattice

The Lieb lattice has three sites per unit cell as illustrated in Fig. S1. We label the sites A,B and C and describe the polariton field on site $j$ (where $j = \mathrm{A, B, C}$) of the unit cell at row $m$ and column $n$ using $\psi_{m,n}^{(j,H)}$ for the horizontal polarisation and $\psi_{m,n}^{(j,V)}$ for the vertical polarisation. Here horizontal and vertical mean with electric field mostly along the $x$ and $y$ directions respectively. The unit cell column (row) indexes run from 0 to $N_x$ ($N_y$) where $N_x$ and $N_y$ are the number of unit cells in the two directions. The physical coordinates of the A lattice sites are given by

$$x_\mathrm{A} = a_x \left(n - N_x/2\right) \tag{S1a}$$

$$y_\mathrm{A} = a_y \left(m - N_y/2\right) \tag{S1b}$$

Here $a_x$ and $a_y$ are the lattice constants in the $x$ and $y$ directions. In our lattice $a_x = a_y = 2d$ where $d = 2.85$ µm is the distance between adjacent pillars. The coordinates of the B and C lattice sites are given by $x_\mathrm{B} = x_\mathrm{A}$, $y_\mathrm{B} = y_\mathrm{A} - d$, $x_\mathrm{C} = x_\mathrm{A} + d$ and $y_\mathrm{C} = y_\mathrm{C} - d$.

Taking into account hopping between nearest neighbour pillars, external driving from the resonant pump laser, dissipation, and interactions between the polaritons the time evolution

* p.m.walker@sheffield.ac.uk

of the field on each pillar in the lattice (apart from those at the edges, which will have modified couplings as discussed below) can be described by the set of equations.

$$\begin{aligned} i\left(\partial\psi_{m,n}^{(A,H)}/\partial t\right) &= \left(\omega_A - i\gamma_{\mathrm{A}}/2\right)\psi_{m,n}^{(A,H)} + t_{TE}\psi_{m,n}^{(B,H)} + t_{TE}\psi_{m+1,n}^{(B,H)} \\ &+ i\left(\gamma_p/2\right)P_{m,n}^{(A,H)}(x,y,t)e^{-i\omega_p t} \\ &+ \omega_{m,n}^{A,BS}\psi_{m,n}^{(A,H)} - i\omega_{m,n}^{A,Z}\psi_{m,n}^{(A,V)} \end{aligned} \tag{S2a}$$

$$\begin{aligned} i\left(\partial\psi_{m,n}^{(B,H)}/\partial t\right) &= \left(\omega_B - i\gamma_{\mathrm{B}}/2\right)\psi_{m,n}^{(B,H)} \\ &+ t_{TE}^{*}\psi_{m,n}^{(A,H)} + t_{TE}^{*}\psi_{m-1,n}^{(A,H)} + t_{TM}\psi_{m,n}^{(C,H)} + t_{TM}\psi_{m,n-1}^{(C,H)} \\ &+ i\left(\gamma_p/2\right)P_{m,n}^{(B,H)}(x,y,t)e^{-i\omega_p t} \\ &+ \omega_{m,n}^{B,BS}\psi_{m,n}^{(B,H)} - i\omega_{m,n}^{B,Z}\psi_{m,n}^{(B,V)} \end{aligned} \tag{S2b}$$

$$\begin{aligned} i\left(\partial\psi_{m,n}^{(C,H)}/\partial t\right) &= \left(\omega_C - i\gamma_{\mathrm{C}}/2\right)\psi_{m,n}^{(C,H)} + t_{TM}^{*}\psi_{m,n}^{(B,H)} + t_{TM}^{*}\psi_{m,n+1}^{(B,H)} \\ &+ i\left(\gamma_p/2\right)P_{m,n}^{(C,H)}(x,y,t)e^{-i\omega_p t} \\ &+ \omega_{m,n}^{C,BS}\psi_{m,n}^{(C,H)} - i\omega_{m,n}^{C,Z}\psi_{m,n}^{(C,V)} \end{aligned} \tag{S2c}$$

$$\begin{aligned} i\left(\partial\psi_{m,n}^{(A,V)}/\partial t\right) &= \left(\omega_A - i\gamma_{\mathrm{A}}/2\right)\psi_{m,n}^{(A,V)} + t_{TM}\psi_{m,n}^{(B,V)} + t_{TM}\psi_{m+1,n}^{(B,V)} \\ &+ i\left(\gamma_p/2\right)P_{m,n}^{(A,V)}(x,y,t)e^{-i\omega_p t} \\ &+ \omega_{m,n}^{A,BS}\psi_{m,n}^{(A,V)} + i\omega_{m,n}^{A,Z}\psi_{m,n}^{(A,H)} \end{aligned}$$

$$\begin{aligned} i\left(\partial\psi_{m,n}^{(B,V)}/\partial t\right) &= \left(\omega_B - i\gamma_{\mathrm{B}}/2\right)\psi_{m,n}^{(B,V)} \\ &+ t_{TM}^{*}\psi_{m,n}^{(A,V)} + t_{TM}^{*}\psi_{m-1,n}^{(A,V)} + t_{TE}\psi_{m,n}^{(C,V)} + t_{TE}\psi_{m,n-1}^{(C,V)} \\ &+ i\left(\gamma_p/2\right)P_{m,n}^{(B,V)}(x,y,t)e^{-i\omega_p t} \\ &+ \omega_{m,n}^{B,BS}\psi_{m,n}^{(B,V)} + i\omega_{m,n}^{B,Z}\psi_{m,n}^{(B,H)} \end{aligned} \tag{S2d}$$

$$\begin{aligned} i\left(\partial\psi_{m,n}^{(C,V)}/\partial t\right) &= \left(\omega_C - i\gamma_{\mathrm{C}}/2\right)\psi_{m,n}^{(C,V)} + t_{TE}^{*}\psi_{m,n}^{(B,V)} + t_{TE}^{*}\psi_{m,n+1}^{(B,V)} \\ &+ i\left(\gamma_p/2\right)P_{m,n}^{(C,V)}(x,y,t)e^{-i\omega_p t} \\ &+ \omega_{m,n}^{C,BS}\psi_{m,n}^{(C,V)} + i\omega_{m,n}^{C,Z}\psi_{m,n}^{(C,H)} \end{aligned} \tag{S2e}$$

Here $\omega_j$ and $\gamma_j$ are the on-site energies and loss rates respectively on the $j$ = A,B,C sublattices and $t_{TE}$ and $t_{TM}$ are the hopping rates for the cases where the polarisation is aligned perpendicular and parallel to the hopping direction respectively. $P_{m,n}^{(j,k)}$ is the $k$ polarised components of the external pump on site $j$ of row $m$ column $n$. The external pump has a slowly varying temporal envelope around frequency $\omega_p$. The coupling rate of the external pump to the internal cavity field is $\gamma_p$. The terms giving the nonlinear interactions (in the

linear polarisation basis) are defined as follows

$$\omega_{m,n}^{j,BS} = (g_1/2 + g_2/2)\left(\left|\psi_{m,n}^{(j,H)}\right|^2 + \left|\psi_{m,n}^{(j,V)}\right|^2\right) \tag{S3a}$$

$$\omega_{m,n}^{j,Z} = (g_1 - g_2)\,\Im\left(\psi_{m,n}^{(j,H)*}\psi_{m,n}^{(j,V)}\right) \tag{S3b}$$

Here $\omega_{m,n}^{j,BS}$ is the polarisation independent frequency renormalisation (or blueshift) on site $j$ of row $m$ column $n$ while $\omega_{m,n}^{j,Z}$ is the Zeeman-like energy splitting arising from the spin dependence of polariton interactions. $g_1$ ($g_2$) is the interaction constant for polaritons with the same (opposite) circular polarisations. The symbol $\Im$ denotes taking the imaginary part while the superscript $*$ denotes complex conjugation.

### B. Bandstructure and Linear Eigenfunctions

In the absence of nonlinearity ($g_1 = g_2 = 0$) and external drive ($P_{m,n}^{(j,H)} = P_{m,n}^{(j,V)} = 0$ for all $j, m, n$) and for an infinitely repeating lattice ($N_x = N_y = \infty$) Eqns. (S2) may be solved using a Fourier transform. The resulting equations were described and analysed in the supplementary information of Ref.[1]. In slightly different notation the equations for the evolution of the horizontal polarisation take the form

$$i\frac{\partial}{\partial t}\begin{pmatrix}\psi_A(t,\boldsymbol{k})\\ \psi_B(t,\boldsymbol{k})\\ \psi_C(t,\boldsymbol{k})\end{pmatrix} = (\mathcal{H}_{\mathrm{on-site}} + \mathcal{H}_{\mathrm{intra-cell}} + \mathcal{H}_{\mathrm{inter-cell}})\begin{pmatrix}\psi_A(t,\boldsymbol{k})\\ \psi_B(t,\boldsymbol{k})\\ \psi_C(t,\boldsymbol{k})\end{pmatrix} \tag{S4a}$$

$$\mathcal{H}_{\mathrm{on-site}} = \begin{pmatrix}\omega_A - i\gamma_A/2 & 0 & 0\\ 0 & \omega_B - i\gamma_B/2 & 0\\ 0 & 0 & \omega_C - i\gamma_C/2\end{pmatrix} \tag{S4b}$$

$$\mathcal{H}_{\mathrm{intra-cell}} = \begin{pmatrix}0 & t_{TE} & 0\\ t_{TE}^* & 0 & t_{TM}\\ 0 & t_{TM}^* & 0\end{pmatrix} \tag{S4c}$$

$$\mathcal{H}_{\mathrm{inter-cell}} = \begin{pmatrix}0 & t_{TE}e^{ik_y a_y} & 0\\ t_{TE}^* e^{-ik_y a_y} & 0 & t_{TM}e^{ik_x a_x}\\ 0 & t_{TM}^* e^{-ik_x a_x} & 0\end{pmatrix} \tag{S4d}$$

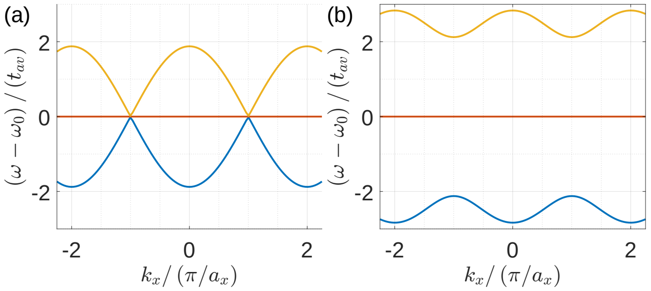


**Supplementary Figure** S2. Energy vs. wavevector bands of the Lieb lattice. (a) Section through $k_y = \pi/a_y$. (b) Section through $k_y = 0$.

Here $\boldsymbol{k} = (k_x, k_y)$ is the wavevector defined over a square first Brillouin zone with $k_x$ from $-\pi/a_x$ to $\pi/a_x$ and $k_y$ from $-\pi/a_y$ to $\pi/a_y$. We note that since there is no nonlinearity the horizontal and vertical polarisations are decoupled and may be solved separately. The equations for the vertical polarisation components are the same but with the symbols $t_{TE}$ and $t_{TM}$ swapped. Inserting a harmonic time dependence ansatz $\psi_s(t, \boldsymbol{k}) = \psi_s(\boldsymbol{k}) \exp(-i\omega t)$ for $s = A, B, C$ we obtain a 3x3 matrix eigenvalue problem which has 3 eigenvalues at each momentum $\boldsymbol{k}$. The eigenvalues and eigenvectors were given in analytic form in Ref. [1].

In the experimentally relevant case where $\omega_A = \omega_B = \omega_C = \omega_0$ and $\gamma_A = \gamma_B = \gamma_C = \gamma$ the frequencies $\omega$ are obtained from $\omega = \lambda + \omega_0 - i\gamma/2$ where $\lambda$ is the solutions of the cubic equation

$$\lambda \left[2\left|t_{TE}\right|^2 (1 + \cos(k_y a_y)) + 2\left|t_{TM}\right|^2 (1 + \cos(k_x a_x)) - \lambda^2\right] = 0 \tag{S5}$$

The three solutions can then be seen from inspection

$$\omega = \omega_0 - i\gamma/2 \tag{S6a}$$

$$\omega = \omega_0 - i\gamma/2 + 2\sqrt{\left|t_{TE}\right|^2 (1 + \cos(k_y a_y))/2 + \left|t_{TM}\right|^2 (1 + \cos(k_x a_x))/2} \tag{S6b}$$

$$\omega = \omega_0 - i\gamma/2 - 2\sqrt{\left|t_{TE}\right|^2 (1 + \cos(k_y a_y))/2 + \left|t_{TM}\right|^2 (1 + \cos(k_x a_x))/2} \tag{S6c}$$

For this case Figure S2 shows the real part of $\omega$. This corresponds to the energy vs. wavevector bandstructure of the lattice, and we have plotted the first two Brillouin zones. The particular parameters used for this plot are $\gamma = 0.25$ meV, $t_{TE} = 0.20$ meV and $t_{TM} = 0.22$ meV. Three distinct bands are present. One always has energy $\hbar\omega_0$ independent

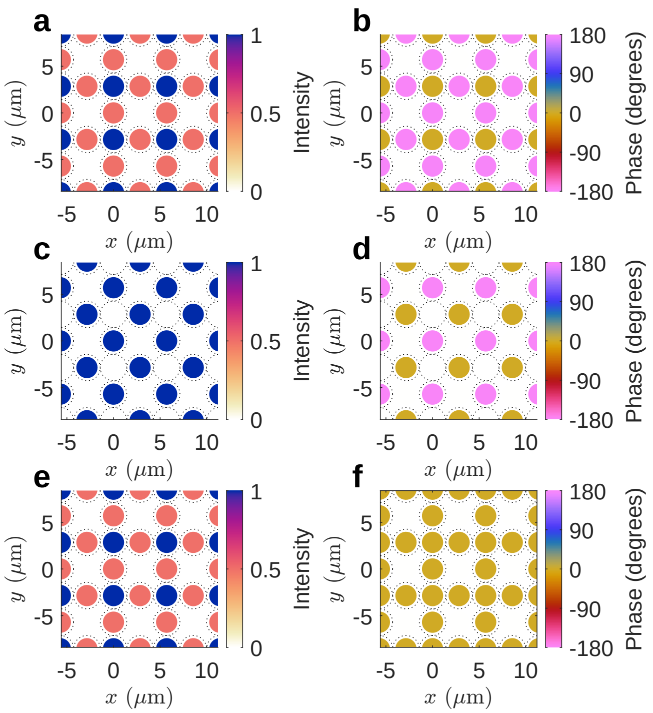


**Supplementary Figure** S3. Sections of the eigenstates of the three bands at $k_x = k_y = 0$ for an infinite size lattice. The left column (a,c,e) shows the intensity (square magnitude of the wavefunction). The right column (b,d,f) shows the phase of the wavefunction. The top (a,b), middle (c,d) and bottom (e,f) rows show the eigenstates corresponding to the lower energy dispersive, flat, and higher energy dispersive bands respectively.

wavevector. We refer to this as the flat band. The other two are mirror-symmetric about $\hbar\omega_0$ and their energy varies with wavevector so that we refer to them as the dispersive bands. At the four corners of the first Brillouin zone (M-points) $|k_x| = \pi/a_x, |k_y| = \pi/a_y$ the dispersive bands come together and touch the flat band at a Dirac point, which can be seen more clearly in the section through $k_y = \pi/a_y$ shown in Fig. S2a.

### C. Eigenvectors

Figure S3 shows the eigenstates corresponding to the three bands for $k_x = k_y = 0$. The dispersive bands (top row and bottom row) have higher intensity on the B sites compared to the A and C sites ((Fig. S3 panels a and e). For the lower energy dispersive band (top row) the B sites are out of phase with the A and C sites by $\pi$ (Fig. S3b) whereas for the higher energy dispersive band (bottom row) all sites are in phase (Fig. S3f). For the flat

band (middle row) the A and C sites have the same intensity while there is no intensity on the B sites (Fig. S3c). The A and C sites are out of phase by $\pi$ (Fig. S3d). For analytical expressions giving the wavevector dependent eigenfunctions see the supplementary materials of Ref. [1].

### D. Nonlinear steady state solutions

To find the steady state solutions in the presence of nonlinearity and external drive we time-integrated Eqns. (S2) in real space on a lattice with $N_x = N_y = 16$. The integration algorithm we used was the MATLAB ode45 solver, which is an implementation of a variable time-step fully explicit fourth order Runge-Kutta method. The initial condition was zero field on all sites. The boundary conditions were fixed by setting zero coupling coefficients to pillars for which $N_y < m < 0$ or $N_x < n < 0$, e.g. for pillars which are not in the lattice. This results in simulation of a finite lattice with dangling bonds at the top and right edges, as depicted in Fig. S1. This is the same configuration as the experimentally measured lattice. We checked that the boundary conditions did not affect the solution by reducing the lattice size to $N_x = N_y = 8$ and seeing that the solution did not change. This occurs because the dissipation prevents propagation to and reflection from the boundaries.

The on-site energy of all pillars was taken as $\omega_j = 0$, resulting in the flat band being at $E = 0$. The loss rate on all pillars $\gamma_j = 0.25$ meV. The hopping rates $t_{TE} = 0.20$ meV and $t_{TM} = 0.22$ meV were obtained from the independently measured photoluminescence spectrum (see Fig. 1c in the main text).

The product $\gamma_p g_1$ of nonlinear strength and pump coupling rate was set so that, in the limit of low pump intensity, circularly polarised and zero-detuned pumping of a single isolated (uncoupled) pillar produced a blueshift of 0.4 meV per unit pump intensity. We also take $g_2 = -0.1 g_1$ as is common in polariton microcavities with GaAs-based quantum wells at negative detunings. For the linear polarised pumps used in this work the nonlinear interaction will be 0.45 times that for a circular polarised field.

The pump spatial and temporal distributions can be seen in Fig. S4. The spatial distribution used for the numerical results presented in the figures in the main text is shown in Fig. S4(a). It was an equal intensity, in-phase, horizontally linearly polarised excitation of the C sites of cells $(m = N_y/2, n = N_x/2)$ and $(m = 1 + N_y/2, n = N_x/2)$, corresponding to

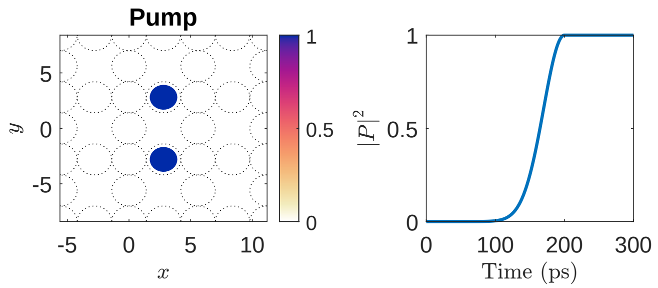


**Supplementary Figure** S4. Excitation condition used in the simulations presented in the figures in the main text. (a) Intensity distribution in space. (b) Intensity vs. time.

the experimental excitation. The time-dependence of the pump is shown in Fig. S4(b). The envelope rises as one half of a 100 ps FWHM Gaussian function to a peak 200 ps after the start of the simulation and then maintains a constant value for 100 ps ($>$ 30x longer than the polariton lifetime) to allow the fields to stabilise at the steady state solution. The pump spectral power density falls to 1% of the peak within a bandwidth of $\pm$0.05 meV.

For the detuning dependence shown in Fig. 2 in the main text a range of pump frequency detunings relative to the flat band were studied. These were calculated using a pump power of $10^{-6}$ so that the nonlinear potential energy (below 1 nano-eV) was negligible compared to linewidth. We thus obtained solutions for the non-interacting regime. For the nonlinear simulations shown in Figs. 3 and 4 in the main text the pump frequency $\omega_p$ was detuned 0.25 meV above the flat band frequency as in the experiment.

## Supplementary Discussion 2. Results for different pump conditions

It is of interest to consider what happens with different spatial configurations of the incident pump laser. In particular, Ref. [2] considered localisation in the non-interacting regime due to pumping multiple adjacent sites. The effect of nonlinearity on these effects was recently discussed theoretically in Ref. [3]. To study these aspects experimentally we therefore shifted our pump spot one column to the left so that it overlapped one A site and the B sites above and below. Fig. S5(a) shows the resulting spatial pattern for powers where the nonlinear interactions are negligible. The site overlapped by the center of the elliptical pump spot, where the pump is brightest, has the highest intensity. The population extends out into the lattice around this spot. The corresponding IPR given in Fig. S5(d) is $\sim$0.3,

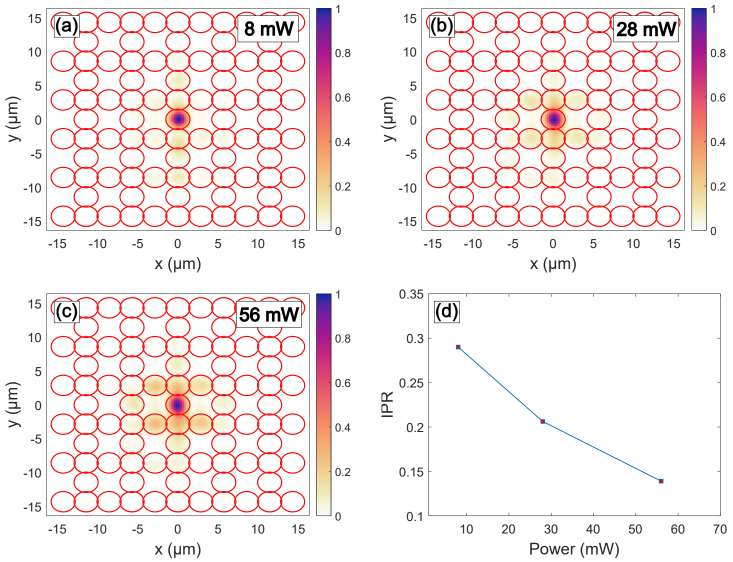


**Supplementary Figure** S5. (a-c) Spatial emission profile when pumping a column of pillars for three powers and a fixed energy detuning of $\Delta E = 0.25$ meV. Intensity is normalised in all images. (d) IPR vs. power.

much below the value of 1 which would be obtained if only a single site were occupied. As the power is increased the population spreads further from the pumped sites, quantified by a reducing IPR. Thus in this case the interactions de-localise the population, in contrast to the pump spatial configuration discussed in the main text.

Figure S6 shows the results of the numerical modeling of this pumping configuration. We achieve a qualitative agreement when the B sites are pumped with intensity 3% that of the A site and out of phase by $\pi$. This pump configuration may arise from the complicated propagation of the tightly focused pump spot through the partially etched semiconductor multilayer structure, which is not easy to model. In the non-interacting regime the out-of-phase pumping on the B sites increases the IPR to 0.28 compared to ∼0.17 for pumping only the A site (see Fig. S7). Stronger out of phase pumping on the B sites increases the localisation on the A site. This is consistent with the driven-dissipative localisation effect reported in Ref. [2]. Because of the relatively strong localisation at low power, when we increase the power the IPR decreases and the field becomes more de-localised. We note that when the B sites are pumped in phase with the A site (see Fig. S10) the low power IPR is lower than for pumping only the A site (Fig. S7) and then increases with increasing power, the opposite to the case here. Thus, the behaviour for pumping a column of pillars

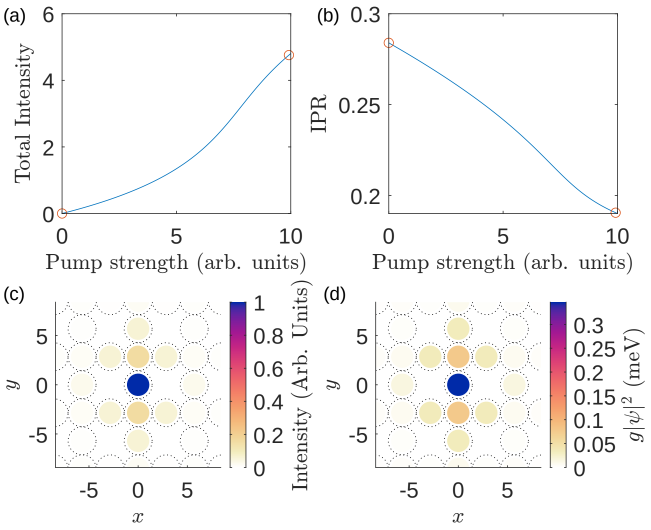


**Supplementary Figure** S6. Simulation results when exciting a column of three pillars. The two outermost pillars are pumped with 3% intensity compared to the central pillar, and out of phase by $\pi$. (a) Total polariton intensity vs. pump power. (b) Inverse participation ratio vs. power. Orange circles indicate the powers at which spatial distributions a plotted. (c,d) Spatial distribution of total intensity on each pillar for the low (c) and high (d) powers indicated by orange circles in (a-b). Color bars give the intensity multiplied by the interaction constant $g$ for linearly polarised polaritons. This is the size of the nonlinear potential energy on each pillar.

depends on the details of the relative pump intensity and phase among the pillars. The nonlinearity can either increase or decrease the localisation depending on whether the low power localisation is low or high.

We now consider numerical simulations of a variety of further pump spatial configurations. In all cases the lattice parameters are as previously described and the laser detuning above the flatband is 250 μeV as before.

Figure S7 shows the case for pumping a single A site on the lattice. The directly pumped pillar is bright and there is some population on the surrounding pillars due to polaritons propagating in the dispersive bands. With increasing pump power the total intensity on the lattice increases gradually while the IPR also increases gradually indicating a slowly increasing localisation.

Figure S8 shows the case for pumping a single C site on the lattice. The results are very similar to those when pumping a single A site, except rotated by 90 degrees. This is expected since the A and C sites in the Lieb lattice are equivalent apart from this rotation.

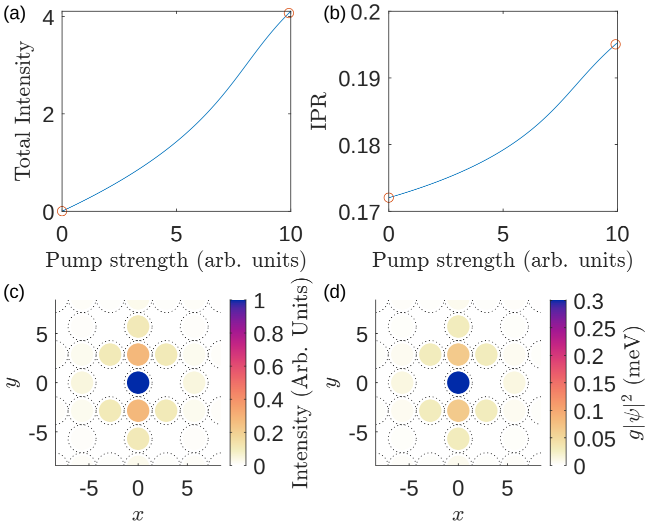


**Supplementary Figure** S7. Simulation results when pumping a single A site. (a) Total intensity vs. pump power. (b) IPR vs. pump power. Orange circles indicate the powers at which spatial distributions a plotted. (c,d) Spatial distribution of total intensity on each pillar for the low (c) and high (d) powers indicated by orange circles in (a-b). Color bars give the intensity multiplied by the interaction constant $g$ for linearly polarised polaritons. This is the size of the nonlinear potential energy on each pillar.

Small numerical differences in the IPR arise because we use horizontally polarised pumping for both Fig. S7 and Fig. S8 and there is a slight difference between $t_{\mathrm{TE}}$ and $t_{\mathrm{TM}}$, the hopping parameters for polarisation aligned perpendicular and parallel to the propagation direction respectively. This causes slightly greater hopping out of the pumped site into the B sites above and below the pumped site, and hence a lower IPR compared to Fig. S7 where the B sites are above and below the pumped site.

Figure S9 shows the case for pumping a single B site on the lattice. This case is interesting since it has zero overlap with the compact localised states, which always have zero population on the B sites. For increasing power the total intensity on the lattice increases slightly sub-linearly. The IPR is initially low and decreases further with increasing power indicating further de-localisation. This indicates that when only the dispersive bands are pumped the repulsive nonlinearity causes defocussing and poorer overlap with the pump. That is the opposite of what we see in Fig. 3 in the main text indicating that our experimental results come mainly from pumping compacton states.

Figure S10 shows the case with a similar pump condition to Fig. S6 except that the B

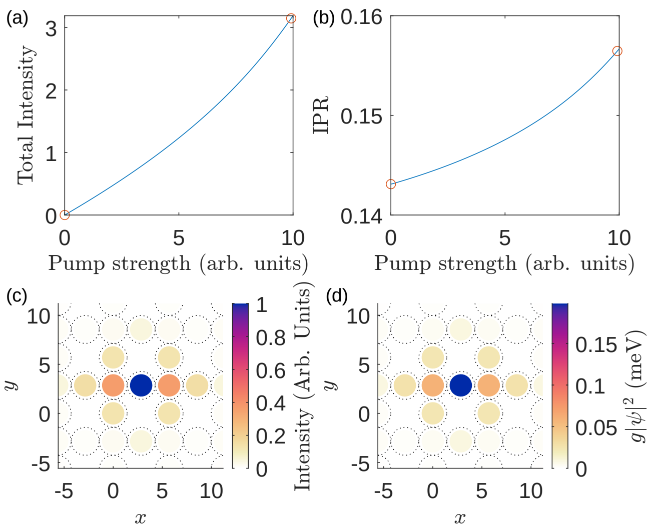


**Supplementary Figure** S8. Simulation results when pumping a single C site. (a) Total intensity vs. pump power. (b) IPR vs. pump power. Orange circles indicate the powers at which spatial distributions a plotted. (c,d) Spatial distribution of total intensity on each pillar for the low (c) and high (d) powers indicated by orange circles in (a-b). Color bars give the intensity multiplied by the interaction constant $g$ for linearly polarised polaritons. This is the size of the nonlinear potential energy on each pillar.

sites are pumped in phase with the A site. Here, at low power, the driving of the B sites delocalises the field more compared to the case of driving the A site only (Fig. S7). This contrasts with Fig. S6 where pumping the B sites out of phase increases localisation. It is clear that for these cases the initial pumping condition greatly affects the initial degree of localisation, in agreement with Ref. [2]. At increased power the IPR approaches a value just below 0.2 for pump power of 10 in all three cases. Depending on the initial IPR this can either be an increase or a decrease.

Figure S11 shows the case where the pump has the profile of an ideal compact localised state, e.g. two A sites and two C sites on a single plaquette, all equally excited but with the C site pumps out of phase with the A site pumps by $\pi$. This case is interesting because it has maximal (minimal) overlap with the non-interacting regime compact localised state (dispersive bands). The solution at low power is highly localised with IPR $\sim$0.25 as expected for an ideal compact localised state. There is a slight difference in intensity between the A and C sites due to the different hopping coefficients $t_{\text{TE}}$ and $t_{\text{TM}}$ (see Ref. [1]). With increasing power there is a sudden jump in the total intensity on the lattice, qualitatively

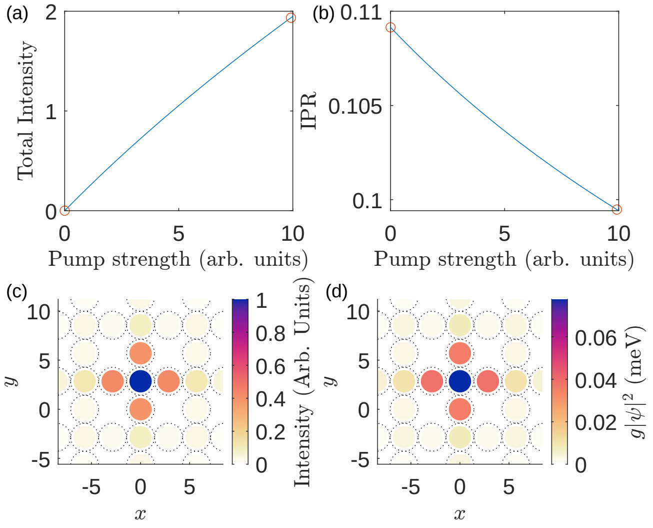


**Supplementary Figure** S9. Simulation results when pumping a single B site. (a) Total intensity vs. pump power. (b) IPR vs. pump power. Orange circles indicate the powers at which spatial distributions a plotted. (c,d) Spatial distribution of total intensity on each pillar for the low (c) and high (d) powers indicated by orange circles in (a-b). Color bars give the intensity multiplied by the interaction constant $g$ for linearly polarised polaritons. This is the size of the nonlinear potential energy on each pillar.

similar to effects seen for states of isolated pillars. Although there is a jump in the IPR at the same threshold power the numerical values of the IPR remain within 1% of 0.25. This indicates that the solution remains a highly localised compacton at all powers and, as a result, behaves like an isolated region of the lattice.

## Supplementary Discussion 3. Comparison with other works

We have shown experimentally that in a 2D Lieb lattice, where a flat band is embedded within dispersive bands, nonlinear interactions can create stable localisation into a compacton state. Provided the driving field has sufficient overlap with the linear regime compact localised states there can be a sudden increase in intensity of the compacton above some threshold power. This is reminiscent of the bistable intensity jumps seen when pumping single isolated micropillars [4, 5]. In that case the nonlinearity blueshifts a pillar state further into resonance with the blue-detuned pump thus increasing the pumping efficiency. This leads to a super-linear increase in intensity vs. pump power. A compact localised state

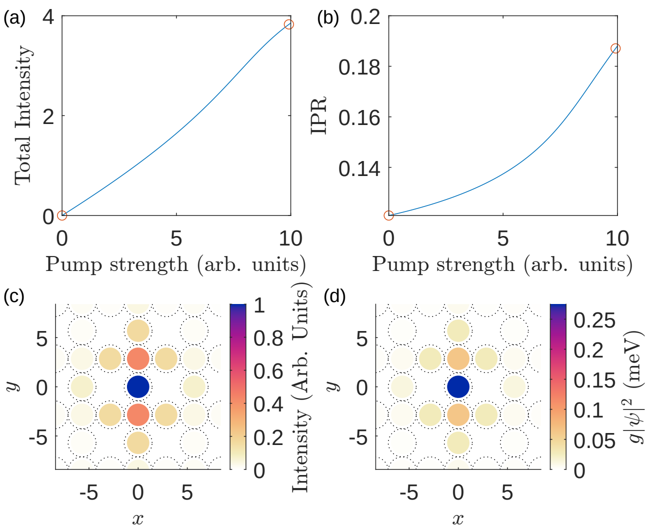


**Supplementary Figure** S10. Simulation results when exciting a column of three pillars all in phase. The two outermost pillars are pumped with 3% intensity compared to the central pillar. (a) Total intensity vs. pump power. (b) IPR vs. pump power. Orange circles indicate the powers at which spatial distributions a plotted. (c,d) Spatial distribution of total intensity on each pillar for the low (c) and high (d) powers indicated by orange circles in (a-b). Color bars give the intensity multiplied by the interaction constant $g$ for linearly polarised polaritons. This is the size of the nonlinear potential energy on each pillar.

is spatially localised and might therefore be expected to behave like a state of an isolated micropillar. However, we have a lattice of coupled pillars and the flat band states are embedded in dispersive bands. The strong spatially localised nonlinear potential breaks the lattice periodicity so that in the general case the bands of the linear regime are not expected to be preserved. Some additional physics is required to explain why the states remain localised at elevated powers.

There is some qualitative similarity between our observations and the gap solitons which have been studied theoretically in many systems. Indeed it was shown that both flat-band and dispersive-band states can transform into gap soliton states when the interaction energy on some lattice sites push them into a band gap of the linear system [6–8]. This was experimentally demonstrated in the driven-dissipative regime for a polariton stub lattice, a one-dimensional analog of the Lieb lattice [9]. In this case the localisation occurs because there are, by definition, no dispersive bands within the gap and so no means to transport energy away. Crucially, however, the gap soliton mechanism does not exist when the flat

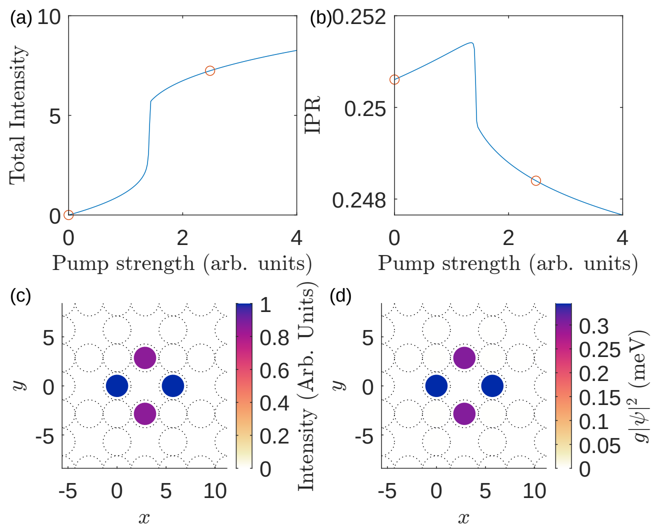


**Supplementary Figure** S11. Simulation results when pumping with the spatial profile of an ideal compact localised state. (a) Total intensity vs. pump power. (b) IPR vs. pump power. Orange circles indicate the powers at which spatial distributions a plotted. (c,d) Spatial distribution of total intensity on each pillar for the low (c) and high (d) powers indicated by orange circles in (a-b). Color bars give the intensity multiplied by the interaction constant $g$ for linearly polarised polaritons. This is the size of the nonlinear potential energy on each pillar.

band is embedded within dispersive bands, as in our case. The color scale on Figs. 4(c) in the main text gives the size of the nonlinear potential energy. It can be seen that the compacton state is well established already for a peak potential of 0.3 meV. This is insufficient to drive flatband states out of the dispersive bands which stretch $\pm 2\sqrt{t_{\text{TE}}^2 + t_{\text{TM}}^2} = \pm\, 0.6$ meV either side of the flat band. Therefore the mechanism responsible for our localised nonlinear states is different from gap soliton formation.

Our results can instead be explained as a preferential population of compact localised discrete soliton (compacton) states [10] as discussed in the main text (Discussion section). We note that Ref. [10] shows that the compacton states are, in a formal sense, unstable at the low powers we study due to resonances with the dispersive bands. However, in our system the polariton linewidth $\sim 1.2 t_{av}$ is higher than the expected instability growth rate $< 0.8 t_{av}$ which, combined with the external pump, may prevent destabilisation. Above a threshold power where the interactions exceed the width of the dispersive bands it is also predicted that the system could jump to single-occupied-site solutions [10], but we did not reach this regime in our experiments.

Lazarides and Tsirones [11] theoretically studied lossless Lieb lattice metamaterials consisting of superconducting quantum interference devices. For excitation of single corner (B) sites they found the nonlinearity leads to delocalisation, as we observe in Fig. S9. For excitation of edge (A or C) sites they also found nonlinear delocalisation. This is in contrast to our numerical results. However, they study a different regime without dissipation or pumping above the flat band energy. At higher powers their initially observed delocalisation was followed by formation of discrete breather solitons, solutions localised purely by nonlinearity rather than by the flat band frustration [12]. Their discrete breathers formed only on the directly pumped sites, and only at powers much higher than those where initial nonlinear effects become apparent. This is qualitatively different to our compacton solutions which form out of the zero power compact localised states.

## Supplementary Discussion 4. Background subtraction and IPR calculation

When calculating the IPR values from experimental data we must first subtract off background CCD counts that do not arise from the actual polariton field inside the cavity. Such counts arise mainly from CCD dark counts, laboratory lights and random laser scatter from lenses, mirrors etc. in the optical path. Since the polariton linewidth is similar to the hopping coefficients the real signal in pillars more than a few hops from the directly pumped pillars must be negligible and due to background only. To calculate a background value for each measurement the average CCD count was taken from pixels in two 50 μm wide regions vertically between 35 μm and 48 μm (12-17 pillars) above and below the pumped pillars.

After subtracting the background we calculate the IPR. Formally, the calculation of IPR involves a sum over all pillars. However, to avoid adding unnecessary noise we sum over a smaller region encompassing the pillars where the intensity is above background level, as well as a few background level pillars surrounding it. This optimises the signal to noise ratio. The 40 pillars used to calculate the IPR are shown as circles on Fig. 2(a-d) and Fig. 3(a-d) in the main text. For each pillar the intensity was measured using the average number of counts from a 3x3 rectangle of CCD pixels at the center of the pillar. This was chosen to avoid including the tails of the spatial Gaussian intensity distribution from adjacent pillars. We checked that including another 2 unit cells in each of the horizontal and vertical direction (additional 56 pillars) in the IPR calculation only changed the absolute values of the IPR by

less than 0.013. This results from inclusion of an excessive number of background counts. Similarly, we checked that increasing the size of rectangle from 3x3 to 5x5 or 7x7 pixels the IPR was not significantly affected. In all cases semi-quantitative agreement with the theory was maintained.

---


[1] Whittaker, C. E. *et al.* Exciton polaritons in a two-dimensional lieb lattice with spin-orbit coupling. *Phys. Rev. Lett.* **120**, 097401 (2018).

[2] Jamadi, O. *et al.* Reconfigurable photon localization by coherent drive and dissipation in photonic lattices. *Optica* **9**, 706–712 (2022).

[3] Muñoz de las Heras, A., Amo, A. & González-Tudela, A. Nonlinearity-enabled localization in driven-dissipative photonic lattices. *Phys. Rev. A* **109**, 063523 (2024).

[4] Boulier, T. *et al.* Polariton-generated intensity squeezing in semiconductor micropillars. *Nature Communications* **5**, 3260 (2014).

[5] Baas, A., Karr, J. P., Eleuch, H. & Giacobino, E. Optical bistability in semiconductor microcavities. *Phys. Rev. A* **69**, 023809 (2004).

[6] Vicencio, R. A. & Johansson, M. Discrete flat-band solitons in the kagome lattice. *Phys. Rev. A* **87**, 061803 (2013).

[7] Johansson, M., Naether, U. & Vicencio, R. A. Compactification tuning for nonlinear localized modes in sawtooth lattices. *Phys. Rev. E* **92**, 032912 (2015).

[8] Beličev, P. P., Gligorić, G., Maluckov, A., Stepić, M. & Johansson, M. Localized gap modes in nonlinear dimerized lieb lattices. *Phys. Rev. A* **96**, 063838 (2017).

[9] Goblot, V. *et al.* Nonlinear polariton fluids in a flatband reveal discrete gap solitons. *Phys. Rev. Lett.* **123**, 113901 (2019).

[10] Real, B. & Vicencio, R. A. Controlled mobility of compact discrete solitons in nonlinear lieb photonic lattices. *Phys. Rev. A* **98**, 053845 (2018).

[11] Lazarides, N. & Tsironis, G. P. Squid metamaterials on a lieb lattice: From flat-band to nonlinear localization. *Phys. Rev. B* **96**, 054305 (2017).

[12] Flach, S. & Gorbach, A. V. Discrete breathers — advances in theory and applications. *Physics Reports* **467**, 1–116 (2008).
